# Supplementary material for: Mathematical Information Retrieval: Search and Question Answering
Source: arXiv:2408.11646 source file (2025-01-14)
Supplement: Supplementary file 3 [file chAppendixB-Exercises.tex]

\chapter{Exercises}
\section{Chapter 2 - Information Needs}
\begin{enumerate}
    \item Consider a mathematical information need. For this information need create three types of queries, one with isolated formula, one with text only, and one with combination of text and formula. Issue these three queries to two search engines: one a general search engine (e.g. Google, Bing, Yahoo, or etc.) and one a math-aware search engine (e.g. Approach0, MathDeck, WebMIaS,or etc.). Compare the top-10 results among the search engines for each of the queries in terms of effectiveness (Precision@10). Is there a search engine that has better effectiveness compared to the others?
    \item There are mathematical formulas that can be associated with a mathematical concept. For example, the formula $a^2+b^2=c^2$, is associated with ``Pythagorean theorem''. Using a general and math-aware search engine, compare the search results obtained when searching with a formula and when searching using a associated concept. Next, use the combination of both text and formula and discuss if the search results improves.
\end{enumerate}

\section{Chapter 3 - User Interfaces}
\begin{enumerate}
    \item Using queries from first exercise in Chapter 2, compare the features for the query interface among a general search engines and a math-aware search engine. Discuss what query interface and search results interface are similar and different. For each search engine, introduce an additional feature that can enhance user interface designs (for query or search results).
\end{enumerate}

\section{Chapter 4 - Formula Indexing} 
\begin{enumerate}
    \item \textbf{Indexing Math Formulas.} There are systems such as Tangent-S\footnote{The link to this system is provided in the resources appendix.} that generate set of tuples over a math formula by doing a depth first traverse on the tree. For example, for the formula $a+b$, the following tuples would be created using SLT (Symbol Layout Tree) and OPT (Operator Tree) as shown in table \ref{tab:ex_slt_opt}.
    
    % A reference to an in-place table \reftab{tab:x}.
    \ourtable{h}{\begin{tabular}{c | c} \hline 
    SLT & OPT \\  
    \hline
    (a, +, n) & (+, a, 0) \\
    (+, b, n) & (+, b, 0) \\ \hline 
    \end{tabular}}{SLT and OPT tuples created for the formula $a+b$.}{tab:ex_slt_opt}
    
    Considering these tuples as the tokens, use ARQMath dataset and create inverted index on SLT and OPT representations of formulas. Discuss the space complexity of the index. 
    
    \item Using the inverted index created from the previous question, apply a compression techniques such as Delta encoding and discuss how it can improves the space complexity.
\end{enumerate}

\section{Chapter 5 - Formula Search}
\begin{enumerate}
    \item Using the inverted index created from the exercise in Chapter 4, consider ARQMath task 2 and use TF-IDF model to search for the formulas. Discuss the effectiveness of the model compared to the runs submitted to the ARQMath lab.
    \item There embedding models for math formulas such as EARN and Tangent-CFT, for which the codes are publicly available. These models convert formulas to a vector representations.   Embedding model. Design a fully-connected neural network that takes in two vector representations of formulas and decide their similarity. For training, you can use the embeddings from one of the current existing models and use ARQMath topics to train the model. Discuss how the model can change the effectiveness of the previous embedding used as the inputs of the fully-connected network.
\end{enumerate}

\section{Chapter 6 - Formula Extraction} 
\begin{enumerate}
    \item TBD
\end{enumerate}

\section{Chapter 7 - Formula + Text Indexing} 
\begin{enumerate}
    \item TBD
\end{enumerate}

\section{Chapter 8 - Formula + Text Search} 
\begin{enumerate}
    \item TBD
\end{enumerate}

\section{Chapter 9 - Evaluation} 
\begin{enumerate}
    \item TBD
\end{enumerate}

\label{c-exercises}
