# Supplementary material for: Mathematical Information Retrieval: Search and Question Answering
Source: arXiv:2408.11646 source file (2025-01-14)
Supplement: Supplementary file 4 [file chAppendixC-Resources.tex]

\chapter{Resources}
\label{c-resources}

\section{MIR Test Collections}
Here we provide a list of 6 known test collection for math-aware search and question answering. For each test collection, we have provided its associated paper, link to the test collection and the defined tasks.
\begin{enumerate}
    \item \textbf{NTCIR-10}
        \begin{itemize}
        \item \textbf{Paper:} NTCIR-10 Math Pilot Task Overview
        \item \textbf{Link:} \url{http://ntcir-math.nii.ac.jp/ntcir10-math/task/}
        \item \textbf{Tasks:} Formula+Text search, Formula search, Math understanding
        \end{itemize}
    \item \textbf{NTCIR-11}
        \begin{itemize}
        \item \textbf{Paper:} NTCIR-11 Math-2 Task Overview
        \item \textbf{Link:} \url{https://ntcir-math.nii.ac.jp/ntcir11-math/task-overview/}
        \item \textbf{Tasks:} Formula+Text search, Formula search (item retrieval)
    \end{itemize}
    \item \textbf{NTCIR-12}
        \begin{itemize}
        \item \textbf{Paper:} NTCIR-12 MathIR Task Overview
        \item \textbf{Link:} \url{https://ntcir-math.nii.ac.jp/data/}
        \item \textbf{Tasks:} Formula+Text search, Formula search
    \end{itemize}
    \item \textbf{SemEval 2019 Task 10}
        \begin{itemize}
        \item \textbf{Paper:} SemEval 2019 Task 10: Math Question Answering
        \item \textbf{Link:} \url{https://github.com/allenai/semeval-2019-task-10}
        \item \textbf{Tasks:} Math question answering
    \end{itemize}
        \item \textbf{ARQMath-1}
        \begin{itemize}
        \item \textbf{Paper:} Overview of ARQMath 2020: Clef Lab on Answer Retrieval for Questions on Math
        \item \textbf{Link:} \url{https://www.cs.rit.edu/~dprl/ARQMath/}
        \item \textbf{Tasks:} Answer retrieval for math questions, Formula search
    \end{itemize}
        \item \textbf{ARQMath-2}
        \begin{itemize}
        \item \textbf{Paper:} Overview of ARQMath-2 (2021): Second CLEF Lab on Answer Retrieval for Questions on Math
        \item \textbf{Link:} \url{https://www.cs.rit.edu/~dprl/ARQMath/}
        \item \textbf{Tasks:} Answer retrieval for math questions, Formula search
    \end{itemize}
\end{enumerate}

\section{Formula Extraction and Recognition Data}
The list below provides link to the open source formula extraction and recognition tools for math:

\begin{enumerate}
    \item \textbf{im2markup} \url{https://github.com/harvardnlp/im2markup}
    \item \textbf{Off-Line Math Formula Recognition Using Deep Neural Networks} \url{https://github.com/jungomi/math-formula-recognition}
    \item \textbf{SmartMath} \url{https://github.com/woshiwpa/SmartMath}
    \item \textbf{MathSeer Extraction} \url{https://www.cs.rit.edu/~dprl/software.html}
\end{enumerate}

\section{Tools for Converting Math Formula Encodings}
This sections lists the existing tools for converting different encodings of math notations.
\begin{enumerate}
    \item \textbf{HeVeA} \url{http://hevea.inria.fr/}
    \item \textbf{latex2mathml} \url{https://github.com/roniemartinez/latex2mathml}
    \item \textbf{\LaTeX ml} \url{https://dlmf.nist.gov/LaTeXML/}
    \item \textbf{Mathoid} \url{https://www.mediawiki.org/wiki/Manual:Mathoid}
    \item \textbf{SnuggleTeX} \url{https://www2.ph.ed.ac.uk/snuggletex/documentation/overview-and-features.html}
    \item \textbf{TeX4ht} \url{https://www.tug.org/tex4ht/}
    \item \textbf{TeXZilla} \url{https://github.com/josephrexme/TeXZilla}
\end{enumerate}

\section{MIR Systems and Code}
In this section, we provide a list of math-aware search system for which the code is available online. Please consider citing the associated papers upon using.
\begin{enumerate}
    \item \textbf{Approach 0.} \url{https://github.com/approach0/pya0}
    \item \textbf{EARN.} \url{https://cse-ai-lab.github.io/MathIR/EARN/}
    \item \textbf{Tangent-CFT.} \url{https://github.com/BehroozMansouri/TangentCFT}
    \item \textbf{Tangent-S.} \url{https://github.com/MattLangsenkamp/tangent-s}
    \item \textbf{Tangent-V.} \url{https://www.cs.rit.edu/~dprl/files/TangentV-source.zip}
    \item \textbf{WebMIaS.} \url{https://github.com/MIR-MU/WebMIaS}
    \item \textbf{WikiMirs.} \url{https://github.com/huxuan/WikiMirs}
\end{enumerate}
