# Supplementary material for: Mathematical Information Retrieval: Search and Question Answering
Source: arXiv:2408.11646 source file (2025-01-14)
Supplement: Supplementary file 5 [file chAppendixA-Notes-Instructors.tex]

\chapter{Notes for Instructors}
\label{c-notes-instructors}

\begin{itemize}
    \item Approaches to presenting/using the book and exercises in courses     
    \begin{itemize}
        \item **Tie back to outline of topics in the Preface.
        \item Intro IR courses (undergrad, grad)
        \item Multimedia retrieval courses
    \end{itemize} 
    \item Notes on exercises
    \item Pertinent instructor resources that might be of help
\end{itemize}
